# Supplementary material for: Towards End-to-End Structure Solutions from Information-Compromised Diffraction Data via Generative Deep Learning
Source: arXiv:2312.15136 source file (2023-12-23)
Supplement: Supplementary file 1 [file supplement.tex]

\section*{Supplemental Information}
